# Supplementary material for: Real-Time Scheduling for 802.1Qbv Time-Sensitive Networking (TSN): A Systematic Review and Experimental Study
Source: arXiv:2305.16772 source file (2024-03-15)
Supplement: Supplementary file 1 [file 8-appendix.tex]

\section{Appendix}

{\cy
\begin{enumerate}
\item Frank et al. (RTNS16\_nw): SMT-NW (SMT with no-wait)
\item Silviu et al. (RTNS16): SMT-WA (Satisfiability Modulo Theories)
\item Ramon et al. (RTAS18): AT (Window-based, Assignment and Array theory) \han{What does R stand for?}
\item Eike et al. (RTNS17): JRS-WA (Jount routing)
\item David et al. (RTNS21): JRS-NW (No-wait joint routing)
\item Jonathan et al. (RTCSA18): JRS-NW-L (No-wait joint routing with Logical indicator)
\item Eike et al. (RTCSA20): JRS-MC (Jount-routing with Multicast)
\item Marek et al. (COR22): LS-TB (List Scheduler with TraceBack)
\item Maryam et al. (SIGBED19): LS (List Scheduler)
\item Xi et al. (JAS21): SMT-FR (SMT with Fragmentation)
\item Ayman et al. (TII20): I-ILP (Iterative-ILP)
\item Marek et al. (CIE21): CP-WA (Constraint Programming)
\item Yuanbin et al. (ASPDAC22): SMT-PR (SMT with Preemption)
\item Xi et al. (ACCESS20): I-SOMT (Iterative-OMT)
\item Jonathan et al. (RTAS20): CG (Conflict-graph)
\item Yanzhou et al. (GLOBECOM22): DT (Divisibility Theory)
\end{enumerate}
}
